# Supplementary material for: CosmoDRAGoN II: Remnant Radio Galaxies in Group and Cluster Environments
Source: arXiv:2511.01193 source file (2025-11-03)
Supplement: Supplementary file 1 [file appendices.tex]

\section{Appendix A - extra plots}

\begin{figure*}
    \centering
    \includegraphics[width=0.8\linewidth]{Figures/extra_low_power_particle_plots.png}
    \caption{Extra `particle mixing' section plots for low-powered progenitors}
    \label{fig:extra low powered particle plots}
\end{figure*}

\section{Appendix B - the magnetic field calculations}

Going through \cite{Shabala_sound_waves_2009} and attempting to re-derive the e-folding time for the Perseus cluster. It's given as $5.5\times10^7$ years.\\

\noindent First, listed quantities for the Perseus cluster: 
\begin{table}[H]
    \centering
    \begin{tabular}{l|l|l}
        parameter & physical meaning & given value/equation  \\
        \hline
        g & gravity outside the bubble &  $=-c^2 (d/\gamma r)$ \\
        d & exponent on density profile & 0.76 \\ 
        c & sound speed & $1.17 \times 10^6$ m/s \\ 
        $\gamma$ & ideal gas adiabatic index & 5/3 \\
        $\lambda$ & wavelength & 11 kpc \\
        B & magnetic field strength & $120 \mu G$ \\ 
        A & some dimensionless constant & eq. below \\
        a & bubble radius & 6 kpc \\
        $n_a$ & number density at bubble surface & 0.116 cm$^{-3}$\\
        $\epsilon$ & fractional amplitude term & 0.1 \\
        $\mu$ & dimensionless thing & 0.3 
    \end{tabular}
    \caption{Table of parameters used in \cite{Shabala_sound_waves_2009} equations}
    \label{tab:Shabala 2009 Perseus parameters}
\end{table}

\noindent Want to determine how long the surface of the bubble will remain stable to instability growth. 

\noindent Given the number density at the bubble surface is 0.116 cm$^{-3}$, the mass density can be found from $rho = n \mu m_p$. For $\mu = 0.6$, $rho = 1.17 \times 10^{-25} g / cm^3 $. Seems reasonable.\\

\noindent The largest wave number for any growing
instability is $k_{crit} = [(\rho_{ICM} - \rho_{bubble})g / \sigma]^{1/2}$. If $\rho_{ICM} >> \rho_{bubble}$ then $k_{crit}$ is effectively $ (\frac{\rho_{ICM}g}{\sigma})^{1/2}$. \\

\noindent The effect of a magnetic field alters the surface tension, $\sigma$, and so we have $\sigma = \frac{B}{2\pi \mu_0 k}$ and I'm assuming that $k$ is a wave number given by, 
$$ k \approx \left(\frac{\omega_b - i\beta}{c} \right) + i \frac{d}{2\gamma} $$

\noindent where $(\omega_b - i\beta) / c \sim 2\pi / \lambda$. \\

\noindent \textbf{OR, more usefully}, $k = A/a$ for $A$ given below. Both approaches yield similar values of the order $10^{-20} m^{-1}$. \\

\noindent To determine the `e-folding' time, $t_e = 1 / \omega_{max}$, we need $\omega_{max} = (-g_{eff} k_{crit})^{1/2}$ with the effective gravity $g_{eff}$, given as a combination of the term due to
the gravitational potential of the well, $g_{grav}$, and the acceleration of the oscillating cocoon  $g_{osc}$. So $g_{eff} = g_{grav} + g_{osc}$. The oscillation term, $g_{osc}$, is given by 
$$ g_{osc} = \frac{c^2}{a} \left[ \frac{A^3}{(A^2 + 1)}\right] \left(\frac{\epsilon^2}{(1 + \epsilon)^{3+2d/\gamma}}\right)\left[2 - \left(\frac{2d}{\lambda}\right)\epsilon \right] $$ 

\noindent $g_{grav}$ is given as $c^2(d/(\gamma r))$. 

\noindent Where it's assumed that the oscillations are effectively undamped in order to explain observations. Therefore, the $A$ parameter is that given in S+A09 Eq. 17 and is,

$$A = \left[\frac{6 - \mu + (36 + \mu^2 + 24\mu)^{1/2}}{2\mu}\right]^{1/2}$$. 

\noindent For $mu = 0.3$, $A \sim 4.5$.

\noindent Now, is the $g_{grav}$ parameter calculated using the equation given in the top row of Table \ref{tab:Shabala 2009 Perseus parameters}? Or is it something else? 

\noindent If we assume that $g=-c^2(d/(\gamma r))$, with values in Table \ref{tab:Shabala 2009 Perseus parameters} and $r$ is some radial distance from the potential well. 

At the moment, calculated values for the e-folding time are given in Fig. \ref{fig:efoldtime}.

\begin{figure}[H]
    \centering
    \includegraphics[width=\linewidth]{Figures/e-folding-time.png}
    \caption{Re-derived values for the e-folding time given in Shabala and Alexander 2009. The value of $5.5\times10^7$ years given in that paper is shown by the grey dashed line.}
    \label{fig:efoldtime}
\end{figure}
